# Supplementary material for: Towards Efficient Quantity Retrieval from Text:An Approach via Description Parsing and Weak Supervision
Source: arXiv:2507.08322 source file (2025-07-14)
Supplement: Supplementary file 1 [file appendix.tex]

% 指标计算
